# Supplementary material for: WOLF: A modular estimation framework for robotics based on factor graphs
Source: arXiv:2110.12919 source file (2022-02-16)
Supplement: Supplementary file 1 [file appendix.tex]

\appendix[Main base classes]
% \appendices
% \section{Main base classes}
\label{sec:base-classes}
